# Supplementary material for: DriveHierarchy: A Benchmark for Diagnosing VLM Driving Capabilities from Open-Loop Understanding to Closed-Loop Execution
Source: arXiv:2609.31814 source file (2026-09-25)
Supplement: Supplementary file 1 [file appendix.tex]

\section{Task Construction Details}
\label{app:task_details}

This appendix provides the implementation-facing details omitted from the main benchmark construction section (Sec.~\ref{sec:drivehierarchy}). We summarize the data sources, task templates, filtering rules, answer spaces, and evaluation metrics used in \textsc{DriveHierarchy}. Our goal is to make the benchmark fully reproducible while keeping the main paper focused on the capability hierarchy itself.

\subsection{Data Sources and Task Mapping}
\label{app:data_sources}

We construct the open-loop benchmark from five public datasets, each chosen for the specific supervision signal it provides.

\begin{table*}[t]
\centering
\small
\caption{Data-source mapping for the open-loop tasks in \textsc{DriveHierarchy}.}
\label{tab:appendix_data_sources}
\begin{tabular}{llll}
\toprule
Dataset & Supervision used & Tasks supported & Role in the hierarchy \\
\midrule
nuScenes & 3D boxes, visibility, attributes, multi-camera streams, ego pose & L1-1, L1-2, L2-1, L2-2, L2-3 & geometry-aware perception, memory, and relation reasoning \\
DRAMA & object descriptions and 2D bounding boxes & L1-3 & language-grounded localization \\
LingoQA & short image-context question-answer pairs & L1-4 & broader situation understanding \\
DriveLM & future-oriented QA with object grounding & L3-1 & instance-grounded future behavior prediction \\
NAVSIM & continuous driving logs and camera sequences & L3-2 & sequence recovery as a planning proxy \\
\bottomrule
\end{tabular}
\end{table*}

The choice of source dataset follows the capability-first philosophy of the benchmark. We do not force all tasks into a single dataset. Instead, we select the dataset whose native annotation structure most directly exposes the intended competency. For example, geometry-sensitive tasks rely on nuScenes because it provides calibrated 3D annotations and ego-pose information, whereas future behavior prediction is drawn from DriveLM because it contains object-grounded predictive QA pairs. This design improves both task fidelity and the interpretability of benchmark outcomes.

\subsection{Task Templates and Construction Rules}
\label{app:task_templates}

\subsubsection{Level 1}

\paragraph{L1-1 Object \& Hazard Recognition.}
This group is built from camera-visible objects in nuScenes. We map fine-grained categories to a compact target taxonomy including \emph{Vehicle}, \emph{Pedestrian}, \emph{Bicycle}, and \emph{Traffic Cone}. Questions are instantiated in three formats:
\begin{itemize}
\item \textbf{Existence:} ``Is there any \texttt{[Category]} visible in \texttt{[Camera]}?''
\item \textbf{Counting:} ``How many \texttt{[Category]}s are visible in \texttt{[Camera]}?''
\item \textbf{State attribute recognition:} ``What is the current status of the nearest \texttt{[Category]} in \texttt{[Camera]}?''
\end{itemize}

We only use camera-visible annotations after geometric visibility filtering. For state recognition, we restrict questions to objects whose attribute tokens can be confidently mapped to a normalized status vocabulary (e.g., moving, stopped, parked for vehicles). Traffic cones are excluded from state questions because they do not admit meaningful dynamic status labels. To avoid oversampling near-duplicate observations, we apply scene-level throttling and sample-level quotas during data generation.

\paragraph{L1-2 Distance Perception.}
Distance questions are also built from nuScenes, using ego pose and object centers to compute target distance. We use three templates:
\begin{itemize}
\item \textbf{Nearest-object distance:} ``What is the distance to the nearest \texttt{[Category]} in \texttt{[Camera]}? Answer in meters.''
\item \textbf{Certain-object distance:} ``In \texttt{[Camera]}, calculate the distance to the \texttt{[Category]} located at pixel coordinates \texttt{[u, v]}. Answer in meters.''
\item \textbf{Distance-bucket counting:} ``How many \texttt{[Category]}s are within the \texttt{[Near/Mid/Far]} range in \texttt{[Camera]}?''
\end{itemize}

Only objects that are visible in the target camera and satisfy projection validity checks are retained. For the nearest-object questions, we choose the closest valid object within a category. For certain-object distance, the target is anchored by projected image coordinates. For distance-bucket counting, the benchmark uses three ranges: \emph{Near}, \emph{Mid}, and \emph{Far}. Buckets with zero valid instances are omitted at construction time in order to keep the task focused on genuine geometric reasoning rather than trivial null answers.

\paragraph{L1-3 Location Questions.}
This task is constructed from DRAMA annotations that pair object-level descriptions with 2D geometry. The template is:
\begin{itemize}
\item \textbf{Language-guided localization:} ``Please locate the object described as: \texttt{[Description]}. Find the bounding box and output \texttt{[xmin, ymin, xmax, ymax]}.'' 
\end{itemize}

We retain only entries with valid image paths, valid box geometry, and usable descriptive text. Samples with missing geometry or invalid scene metadata are discarded. The resulting task isolates the ability to align natural-language descriptions with image regions.

\paragraph{L1-4 Broader Situation Understanding.}
We build this task from LingoQA short-context question-answer pairs. The task requires free-form text generation conditioned on a short image context and a driving-related prompt. In practice, we retain samples whose question semantics reflect current-context situation or ego-action understanding. This yields a broader situation-understanding setting that unifies contextual scene description and ongoing driving behavior characterization. Because the answer space is open-ended, evaluation is performed with a learned text judge rather than exact matching.

\subsubsection{Level 2}

\paragraph{L2-1 Multi-view Memory.}
This task is built from synchronized six-camera observations in nuScenes. The canonical prompt is:
\begin{itemize}
\item \textbf{Cross-view unique counting:} ``Given the six surround-view images at this timestamp, how many unique vehicles are visible in the surrounding environment?''
\end{itemize}

The crucial construction rule is the \emph{overlap trigger}: we only keep samples where at least one object instance is visible in more than one camera. This avoids degenerate cases in which the task can be solved by treating each view independently and simply summing counts. We further restrict the task to valid dynamic vehicle categories and use set-based deduplication over instance identifiers to obtain the ground-truth answer.

\paragraph{L2-2 Temporal Sequence.}
This level contains two temporal-memory tasks under a given viewpoint.
\begin{itemize}
\item \textbf{Temporal counting:} ``Observing the sequence from the current frame over the next short horizon, how many unique vehicles appear in the given view?''
\item \textbf{Temporal status recognition:} ``Focus on the target object in the initial frame. Observing the clip from $t=0$ to $t=T$, how does its state change?''
\end{itemize}

For temporal counting, we extract fixed-length clips and aggregate unique vehicle instances over the time window using instance identifiers. For temporal status recognition, we require a target instance to be visible at the start frame and, when applicable, at the end frame as well. We then compare the start and end attributes to derive either a transition label or a no-change label. To avoid class imbalance, state-transition questions are approximately balanced between positive transitions and no-change cases.

\paragraph{L2-3 Spatial Relations.}
The canonical prompt is:
\begin{itemize}
\item \textbf{Object-to-object spatial relation:} ``In \texttt{[Camera]}, what is the position of object A at \texttt{[u\_A, v\_A]} relative to object B at \texttt{[u\_B, v\_B]}?''
\end{itemize}

We keep only samples in which at least two distinct valid objects are visible in the same camera view. The ground-truth relation is computed from their relative positions in the ego frame and discretized into relation labels such as \emph{Front}, \emph{Rear}, \emph{Left}, \emph{Right}, \emph{Front-Left}, and \emph{Rear-Right}. Distractor choices are sampled from the same relation vocabulary, and the correct option is randomized among the answer candidates.

\subsubsection{Level 3}

\paragraph{L3-1 Instance-grounded Future Behavior Prediction.}
This task is derived from DriveLM predictive QA pairs. We filter questions that explicitly ask about a target's future state, replace dataset-specific object tags with grounded object descriptions, and map raw free-form answers to a normalized answer inventory. The resulting template is:
\begin{itemize}
\item \textbf{Future behavior prediction:} ``What is the future state of the \texttt{[grounded target object]}?''
\end{itemize}

We retain only samples for which both the object grounding and answer normalization are reliable. The final answer space contains discrete behavior options such as going straight, turning, braking to a stop, lane changing, or remaining stationary, and the correct answer is embedded into a randomized multiple-choice set.

\paragraph{L3-2 Sequential Planning.}
This task is built from NAVSIM continuous scenes. We sample $3$--$5$ frames from the same scene, shuffle them, overlay visual labels (e.g., A/B/C/D), and ask the model to recover their correct chronological order. The construction is restricted to clips that satisfy basic motion complexity criteria, including ego motion and turning-related dynamics, in order to avoid trivial static sequences. The task therefore measures whether the model can infer temporal progression from visual evidence rather than relying on appearance alone.

\subsection{Filtering Principles}
\label{app:filtering_rules}

Although each task has its own construction logic, several filtering principles are shared across the benchmark:
\begin{itemize}
\item \textbf{Visibility grounding.} We only construct questions from objects that are valid in the relevant camera or clip, using dataset-specific visibility metadata and geometric projection checks whenever available.
\item \textbf{Ambiguity reduction.} We prefer targets that can be referenced unambiguously, such as the nearest valid object, a target anchored by image coordinates, or an explicitly described instance.
\item \textbf{Duplicate suppression.} We suppress near-duplicate samples within a scene by enforcing scene-level quotas, sample-level caps, stride-based selection, or non-overlapping clip segmentation.
\item \textbf{Answer reliability.} We discard entries when the ground-truth answer depends on unreliable attribute mapping, unresolved object grounding, invalid geometry, or incomplete temporal context.
\item \textbf{Capability-focused difficulty.} We preserve samples that genuinely test the target capability, such as cross-view overlap in L2-1 or sufficient temporal evolution in L2-2 and L3-2.
\end{itemize}

These rules are designed to improve both fidelity and diagnostic value. The benchmark is not intended to maximize raw sample count at any cost; instead, it prioritizes well-grounded questions whose failure modes can be meaningfully interpreted as capability deficiencies.

\subsection{Evaluation Metrics}
\label{app:metrics}

The benchmark combines exact-match metrics for discrete tasks with soft scoring for numeric and structured outputs. This hybrid protocol is intended to preserve interpretability while avoiding overly brittle evaluation on tasks with continuous answers.

\paragraph{Discrete classification.}
For yes/no questions and multiple-choice questions, we use exact match (EM). A correct prediction receives a score of $100$, and an incorrect prediction receives a score of $0$.

\paragraph{Counting.}
For counting tasks, both prediction and ground truth are normalized to non-negative integers. We define the normalized counting error as
\begin{equation}
E_c = \frac{|\hat{y} - y|}{\max(y, c)},
\label{eq:count_error}
\end{equation}
where $y$ is the ground-truth count, $\hat{y}$ is the predicted count, and $c$ is a small stabilizing constant. The final score is obtained through a bounded exponential mapping,
\begin{equation}
S(E) =
\begin{cases}
100, & E \le \tau, \\
100 \exp\!\left(-\frac{E-\tau}{\sigma}\right), & E > \tau,
\end{cases}
\label{eq:unified_numeric}
\end{equation}
followed by clipping to $[0,100]$. This design rewards exact answers while still assigning partial credit to near-miss predictions.

\paragraph{Distance estimation.}
For distance tasks, both prediction and ground truth are normalized to non-negative scalars, and we define a log-ratio error,
\begin{equation}
E_d = \left| \ln \frac{\hat{y} + \epsilon}{y + \epsilon} \right|,
\label{eq:distance_error}
\end{equation}
where $\epsilon$ is a small constant for numerical stability. The final score again uses the bounded exponential mapping in Eq.~\ref{eq:unified_numeric}. Using a log-ratio error prevents large absolute distances from dominating the metric and better reflects proportional geometric accuracy.

\paragraph{Localization.}
For L1-3 location questions, the score is computed as
\begin{equation}
S_{\text{bbox}} = 100 \cdot \mathrm{IoU}(b, \hat{b}),
\end{equation}
where $b$ and $\hat{b}$ denote the ground-truth and predicted bounding boxes, respectively.

\paragraph{Sequential planning.}
For L3-2, we measure the agreement between the predicted and ground-truth orderings using a normalized inversion-based score,
\begin{equation}
S_{\text{seq}} = 100 \cdot (1 - \mathrm{Inv}_{\mathrm{norm}}),
\end{equation}
where $\mathrm{Inv}_{\mathrm{norm}}$ is the normalized Kendall-style inversion count. This metric assigns full credit to the correct ordering and degrades smoothly as the number of pairwise order violations increases.

\paragraph{Broader situation understanding.}
For L1-4, we use a learned semantic judge rather than exact lexical overlap. Specifically, given the question, reference answer, and model response, we query a pretrained Lingo-Judge classifier and use its confidence score as the final quality estimate:
\begin{equation}
S_{\text{lingo}} = 100 \cdot p_{\text{judge}}.
\end{equation}
This choice is necessary because situation understanding is open-ended and cannot be evaluated reliably with exact-match rules.

\paragraph{Implementation defaults.}
Unless otherwise stated, the benchmark uses a fixed default configuration for the numeric scoring functions. For counting, we set $c=1$, $\tau_c=0.05$, and derive $\sigma_c$ from an $E_{50}$ target of $0.20$, i.e.,
\begin{equation}
\sigma_c = \frac{0.20 - 0.05}{\ln 2}.
\end{equation}
For distance estimation, we set $\epsilon=0.1$, $\tau_d=0$, and derive $\sigma_d$ from $E_{50}=\ln 2$, which yields $\sigma_d = 1.0$. These parameters are fixed across all experiments for fairness and are part of the released evaluation code.

\subsection{Remarks on Scope}
\label{app:scope}

The appendix details above should be read as the operational instantiation of the capability hierarchy, not as its replacement. The central methodological contribution of \textsc{DriveHierarchy} remains the explicit hierarchical decomposition of autonomous driving VLM evaluation. The templates, filters, and metrics described here are chosen to faithfully operationalize that decomposition while maintaining reproducibility, answer reliability, and diagnostic interpretability.
